# Supplementary material for: Multithermal-multibaric molecular simulations from a variational principle
Source: arXiv:1811.08253 ancillary file (2019-01-30)
Supplement: Supplementary file 1 [file supplemental_material.pdf]

# Supplemental material to: Multithermal-multibaric molecular simulations from a variational principle

Pablo M. Piaggi and Michele Parrinello
(Dated: November 22, 2018)

## OPTIMIZATION PROCEDURE

The bias potential was expanded in Legendre polynomials. The coefficients in the expansion were optimized using the averaged stochastic gradient descent algorithm[1, 2]. The order of the expansion and the optimization step $\mu$ are specified below for each simulation. The coefficients were updated every 500 time steps, i.e. 1 ps.

## SODIUM

Sodium was simulated using LAMMPS[3] patched with a development version of the PLUMED 2 enhanced sampling plugin[4]. An embedded atom model (EAM) was used to describe the interatomic interactions[5]. A timestep of 2 fs was used to integrate the equations of motion. The temperature was maintained using the stochastic velocity rescaling thermostat[6] with a 0.1 ps relaxation time. We employed an isotropic version of the Parrinello-Rahman[7] barostat with a relaxation time of 1 ps. A system with 250 atoms was simulated.

### Multicanonical

We performed a simulation at constant temperature $T = 500$ K and constant volume $\mathcal{V} = 10.6146$ nm$^3$. We decided to explore the temperature range from 400 K to 600 K in a multicanonical simulation. We employed a step $\mu = 1$ in the optimization procedure. The energy threshold $\epsilon$ was set to 1 $k_B T$. $p(E)$ was updated every 500 steps of the optimization procedure, i.e. every 0.5 ns. The bias potential was constructed using a 20$^{\text{th}}$ order Legendre polynomial expansion. The energy interval in which the Legendre polynomials were defined was $-25000$ kJ/mol $< E < -23500$ kJ/mol.

The simulation had a first stage of 10 ns during which the target distribution $p(E)$ and the coefficients $\boldsymbol{\alpha}$ were optimized. The convergence of the limits of the interval $E_1 - E_2$ of the $p(s)$ is shown in Figure SI-1a) and the evolution of the 20 coefficients $\alpha$ is shown in Figure SI-1b). The optimization procedure converges in around 1-2 ns. The converged $p(E)$ is shown in SI-1c). The $p(E)$ decays to zero with a Gaussian distribution with $\sigma = 50$ kJ/mol.

At a subsequent stage that lasted 40 ns the coefficients were kept constant. The potential energy as a function of time is shown in SI-1d) (blue solid line). It is clear that the sampled distribution of energy corresponds to the converged $p(E)$. We also show in SI-1d) a trajectory in the canonical ensemble at 500 K (orange solid line). As expected, the fluctuations in energy are greatly increased in the multicanonical case. The multicanonical trajectory can be reweighed in order to obtain properties in the interval 400-600 K using,

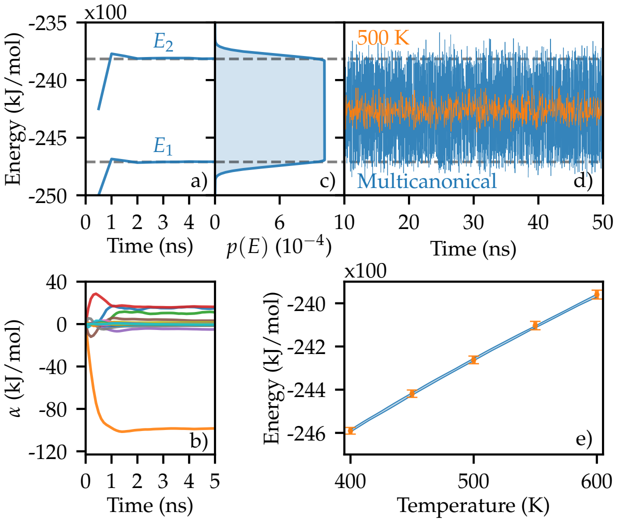


FIG. SI-1. Results of the multicanonical simulation of Na. a) Convergence of the limits of the interval $E_1 - E_2$. The final values of $E_1$ and $E_2$ are shown using a gray dashed line. b) Convergence of the coefficients $\boldsymbol{\alpha}$. c) Converged $p(E)$. d) Potential energy vs. time for the multicanonical simulation (blue solid line) and a canonical simulation at 500 K (orange solid line). e) Mean potential energy for different temperatures. The blue curve are the results obtained from the multicanonical simulation by a reweighting procedure (error is shown as a blue shaded region). The results from individual simulation in the canonical simulations are shown in orange circles with errorbars.

$$\langle O(\mathbf{R}) \rangle_{\beta'} = \frac{\langle O(\mathbf{R}) e^{(\beta-\beta')E(\mathbf{R})} e^{\beta V(E)} \rangle_{\beta,V}}{\langle e^{(\beta-\beta')E(\mathbf{R})} e^{\beta V(E)} \rangle_{\beta,V}} \tag{SI-1}$$

where $\langle \cdot \rangle_{\beta,V}$ is a mean value in the biased ensemble at temperature $\beta$ using a stationary bias potential $V(E)$, and $\langle \cdot \rangle_{\beta'}$ is the mean value in the canonical ensemble at temperature $\beta'$. We used Eq. (SI-1) to calculate the mean potential energies at all temperatures. The results are shown in Figure SI-1e) (blue line) and compared with individual canonical simulations (orange circles with er-

rorbars). The length of each canonical simulations was 1 ns.

### Multibaric

The multibaric version of our method works as follows. We use the volume $\mathcal{V}$ as collective variable and we impose a uniform sampling in the energy interval $\mathcal{V}_1 - \mathcal{V}_2$ by choosing as target distribution:

$$p(\mathcal{V}) = \begin{cases} \frac{1}{\mathcal{V}_2 - \mathcal{V}_1} & \text{if} \quad \mathcal{V}_1 < \mathcal{V} < \mathcal{V}_2 \\ 0 & \text{otherwise} \end{cases}. \tag{SI-2}$$

The limits of the interval are determined as described in the main part for the multitemperature case. In the multibaric version, however, from the knowledge of the free energy as a function of volume at pressure $P$ one can calculate the free energy at a different pressure $P'$ using:

$$F_{P'}(\mathcal{V}) = F_P(\mathcal{V}) + (P' - P)\mathcal{V} + C', \tag{SI-3}$$

where $C'$ is set by the relation $F_{P'}(\mathcal{V}'_m) = 0$. Other details are equivalent to those in the multitemperature case.

We performed a multibaric simulation to explore the pressure interval 0-1GPa. The temperature was maintained at 500 K and the target pressure of the thermostat was 0.5 GPa. The energy threshold $\epsilon$ was set to 5 $k_BT$ although 1 $k_BT$ would have sufficed. The $p(\mathcal{V})$ decays to zero with a Gaussian distribution with $\sigma = 0.05$ nm. The volume interval in which the Legendre polynomials were defined was 8 nm$^3$ $< \mathcal{V} <$ 12 nm$^3$. Other simulation details are the same as described in the multicanonical case.

The optimization stage lasted 10 ns although the simulation was converged after 3-4 ns. Afterwards a simulation of 40 ns was performed with fixed $\boldsymbol{\alpha}$. Using the statistics of the latter simulation we calculated averages at different pressures using:

$$\langle O(\mathbf{R}, \mathcal{V}) \rangle_{P'} = \frac{\langle O(\mathbf{R}, \mathcal{V}) e^{\beta(P-P')\mathcal{V}} e^{\beta V(E)} \rangle_{P,V}}{\langle e^{\beta(P-P')\mathcal{V}} e^{\beta V(E)} \rangle_{P,V}}. \tag{SI-4}$$

In this way, we computed the mean potential energies and volumes between 0 and 1 GPa shown in Figure SI-2. Results from individual isothermal-isobaric simulations are also shown in Figure SI-2 .

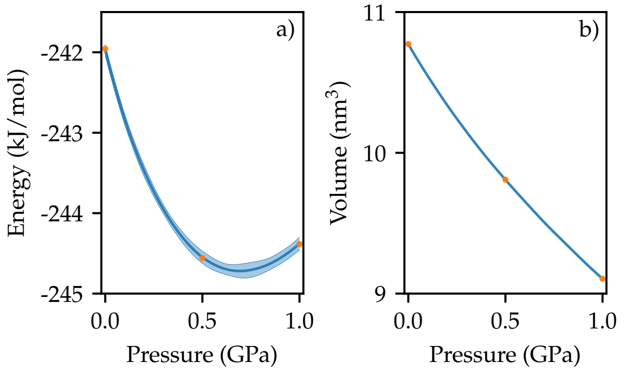


FIG. SI-2. Results of the multibaric simulation of Na. a) Mean potential energy from the multibaric simulation (solid blue line) and references (orange circles). The error is shown as a blue shaded region. b) Mean volume from the multibaric simulation (solid blue line) and references (orange circles). The errors have not been shown in cases where they are too small to be preoperly plotted.

## TIP4P/ICE WATER

MD simulations of TIP4P/Ice water[8] were performed using Gromacs 2018.1[9] patched with a development version of PLUMED 2[4]. Van der Waals and electrostatic interactions in real space were calculated with a 0.85 nm cutoff. The electrostatic interaction in reciprocal space was calculated using the particle mesh Ewald (PME) method [10]. The atomic bonds involving hydrogen were constrained using the LINCS algorithm[11] and the equations of motion were integrated with a 2 fs timestep. The temperature was controlled using the stochastic velocity rescaling thermostat [6] with a relaxation time of 0.1 ps. We maintained the pressure constant employing the isotropic version of the Parrinello-Rahman [7] barostat with a 2 ps relaxation time and a compressibility of 500 mbar. We employed a system composed of 256 water molecules. The reference isothermal-isobaric simulations were run for 100 ns. The multithermal and multithermal-multibaric simulations were performed in two stages. During the first stage the coefficients $\boldsymbol{\alpha}$ of the bias potential were optimized and the $p(\mathbf{s})$ was determined iteratively. These simulations lasted 100 ns, although in some cases the simulations could be considered converged well before this time. During the second stage the coefficients $\boldsymbol{\alpha}$ were kept constant and statistic was gather in 200 ns long simulations.

### Multithermal simulation

A multithermal simulation was performed in order to study the temperature range 260-350 K. The temperature was maintained at 300 K and the target pressure of the barostat was 1 bar. The optimization step was $\mu = 1$ and the $p(E)$ was updated every 0.5 ns. The $p(E)$ decays to zero with a Gaussian distribution with $\sigma = 50$ kJ/mol. The bias potential $V(E)$ was represented using a 20$^{\text{th}}$ order Legendre polynomial expansion. The energy interval in which the Legendre polynomials were defined

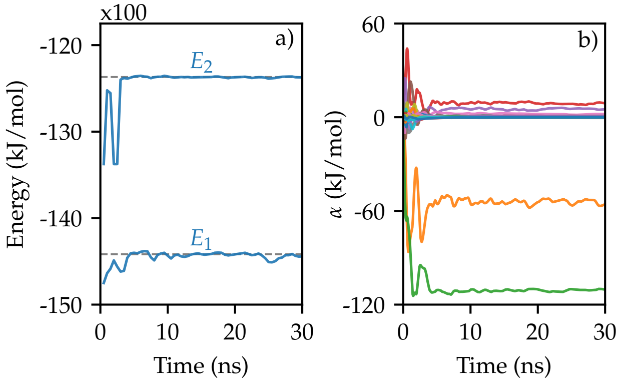


FIG. SI-3. Results of the multithermal simulation of TIP4P/Ice water. a) Convergence of the limits of the energy interval $E_1 - E_2$. b) Convergence of the coefficients $\boldsymbol{\alpha}$.

was $-14750$ kJ/mol $< E < -12000$ kJ/mol.

The results of the optimization are shown in Figure SI-3. Convergence is achieved after $\sim 5$ ns.

### Multithermal-multibaric simulation

A multithermal-multibaric simulation was carried out to study the temperature range 260-350 K and the pressure range 0-300 MPa. The temperature was maintained at 300 K and the target pressure of the barostat was 1 bar. The optimization step was $\mu = 10$ and the $p(E, \mathcal{V})$ was updated every 0.5 ns. $p(E, \mathcal{V})$ was calculated using Eq. (10) of the manuscript. The condition $\beta' F_{\beta',P'}(E, \mathcal{V}) < \epsilon$ was checked in 21 equally spaced points in each dimension $\beta'$ and $P'$. The spacing between points was therefore $\Delta\beta' = 4.5$ K and $\Delta P' = 15$ MPa, and the total number of points 441. The calculation of $p(E, \mathcal{V})$ can be somewhat costly but it is only seldom recalculated (every $2.5 \times 10^5$ MD steps). The boundaries of $p(E, \mathcal{V})$ were smoothened using a Gaussian function with deviation $\sigma_E = 50$ kJ/mol in $E$ and $\sigma_{\mathcal{V}} = 0.05$ nm in $\mathcal{V}$. The bias potential $V(E, \mathcal{V})$ was represented using a $10^{\text{th}}$ order Legendre polynomial expansion in each dimension. The energy and volume intervals in which the Legendre polynomials were defined were $-14750$ kJ/mol $< E < -12250$ kJ/mol and 6.5 nm$^3 < \mathcal{V} < 8.25$ nm$^3$.

The convergence of the coefficients $\boldsymbol{\alpha}$ is shown in Figure SI-4 As in previous cases, the coefficients reach values close to the final ones after a few ns. However, most coefficients stabilized only after 12 ns and a few of them show oscillations even at longer times. Careful observation of the $p(E, \mathcal{V})$ during the optimization process reveals that after a few ns the main features of $p(E, \mathcal{V})$ are already captured. Nonetheless the shape of $p(E, \mathcal{V})$ stabilizes after 50 ns.

It is important to establish whether the bias distribution of $E$ and $\mathcal{V}$ has overlap with the unbiased distribution at the relevant temperatures and pressures. For this reason in Figure SI-5 we represent the regions of the $E - \mathcal{V}$ space sampled in each case. It can be seen that the distributions have good overlap and that the boundaries of the biased distribution are determined relatively well. For low temperatures the determination of the boundary is not perfect and this is a consequence of the optimization procedure that could be improved. However, since the results presented are obtained after reweighting with a static bias potential, these imperfections do not play a significant role.

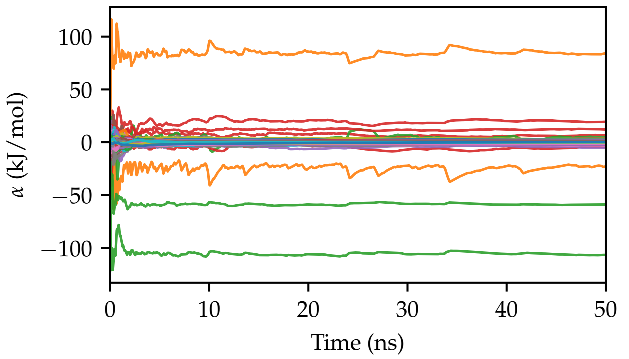


FIG. SI-4. Results of the multithermal-multibaric simulation of TIP4P/Ice water. Convergence of the coefficients as a function of time.

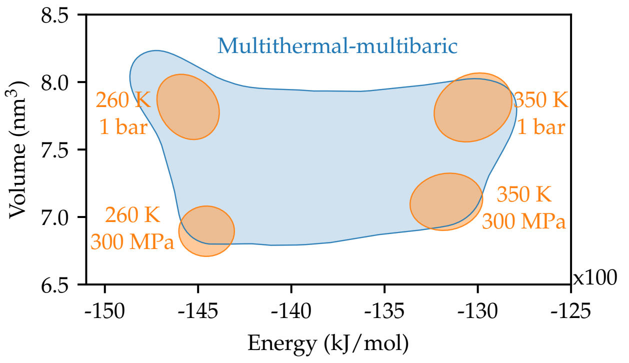


FIG. SI-5. Illustration of the sampled regions of the $E\mathcal{V}$ space in isothermal-isobaric simulations (orange) and multithermal-multibaric (blue). The regions correspond to 5 $k_B T$ contour lines of the free energies.

We also calculated the tetrahedral order parameter described in ref. [12] for all temperatures and pressures. The results are shown in Figure SI-6.

[1] O. Valsson and M. Parrinello, Physical review letters **113**, 090601 (2014).

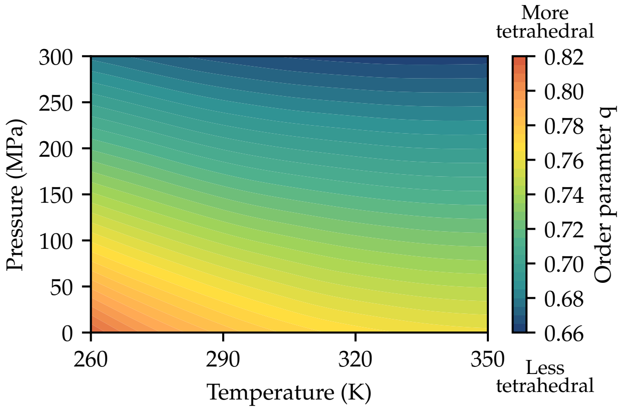


FIG. SI-6. Tetrahedral order parameter for TIP4P/Ice water at different temperatures and pressures. All values were calculated from a single multithermal-multibaric simulation.


[2] F. Bach and E. Moulines, in *Advances in Neural Information Processing Systems* (2013) pp. 773–781.

[3] S. Plimpton, Journal of computational physics **117**, 1 (1995).

[4] G. A. Tribello, M. Bonomi, D. Branduardi, C. Camilloni, and G. Bussi, Computer Physics Communications **185**, 604 (2014).

[5] S. Wilson, K. Gunawardana, and M. Mendelev, The Journal of chemical physics **142**, 134705 (2015).

[6] G. Bussi, D. Donadio, and M. Parrinello, The Journal of chemical physics **126**, 014101 (2007).

[7] M. Parrinello and A. Rahman, Journal of Applied physics **52**, 7182 (1981).

[8] J. Abascal, E. Sanz, R. García Fernández, and C. Vega, The Journal of chemical physics **122**, 234511 (2005).

[9] M. J. Abraham, T. Murtola, R. Schulz, S. Páll, J. C. Smith, B. Hess, and E. Lindahl, SoftwareX **1**, 19 (2015).

[10] U. Essmann, L. Perera, M. L. Berkowitz, T. Darden, H. Lee, and L. G. Pedersen, The Journal of chemical physics **103**, 8577 (1995).

[11] B. Hess, Journal of Chemical Theory and Computation **4**, 116 (2008).

[12] J. R. Errington and P. G. Debenedetti, Nature **409**, 318 (2001).
